# Supplementary material for: Unit Disk Representations of Embedded Trees, Outerplanar and Multi-Legged Graphs
Source: arXiv:2103.08416 source file (2021-08-26)

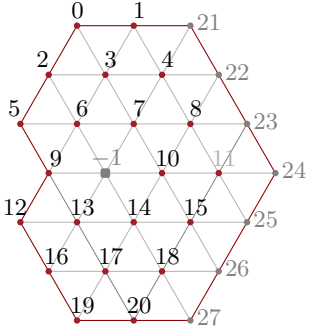

6, 2

6, 5

6, 9

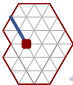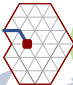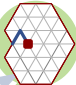

9

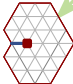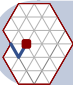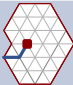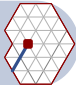

13, 9

13, 12

13, 16



[illegible]
$$7 \wedge 10 \implies 4$$
$$7 \wedge 10 \implies 8$$
$$10 \wedge 14 \implies 15$$
$$14 \wedge 13 \implies 17$$
$$\underline{13} \wedge 9 \implies \underline{12}$$
$$7 \wedge 10 \wedge 14 \implies 11$$
$$10 \wedge 14 \wedge 13 \implies 18$$
$$14 \wedge 13 \wedge 9 \implies 16$$
$$7 \wedge 10 \wedge 14 \wedge 13 \implies 7$$
$$7 \wedge 10 \wedge 14 \wedge 13 \implies 10$$
$$7 \wedge 10 \wedge 14 \wedge 13 \implies 13$$
$$7 \wedge 10 \wedge 14 \wedge 13 \implies 14$$
[illegible]

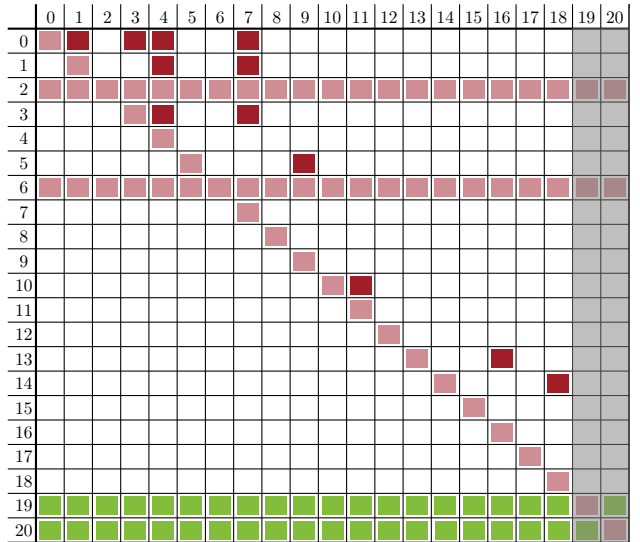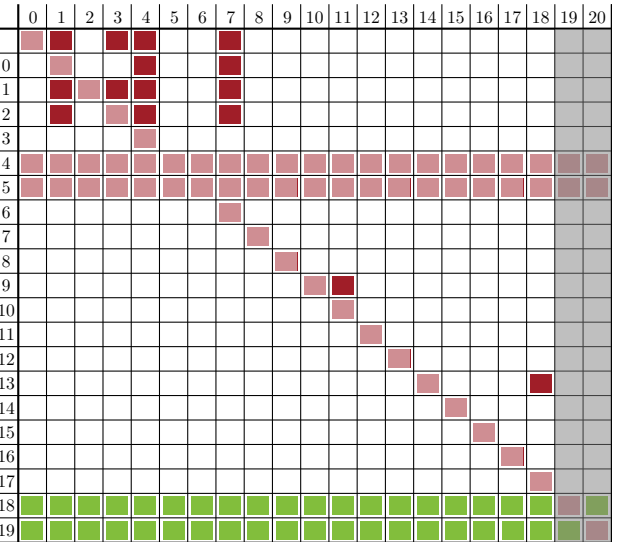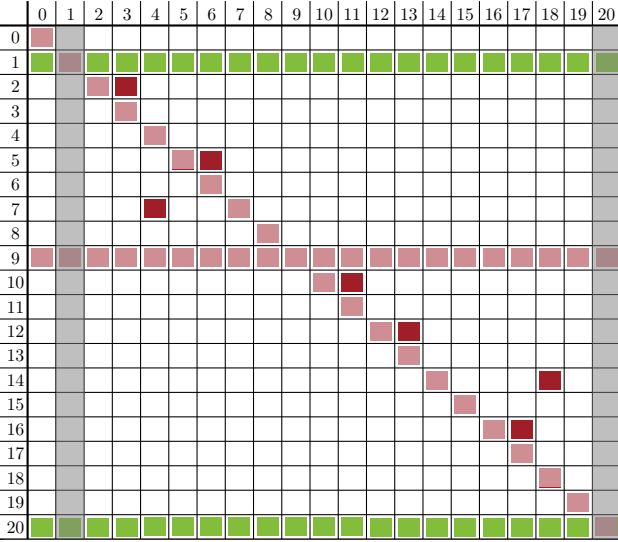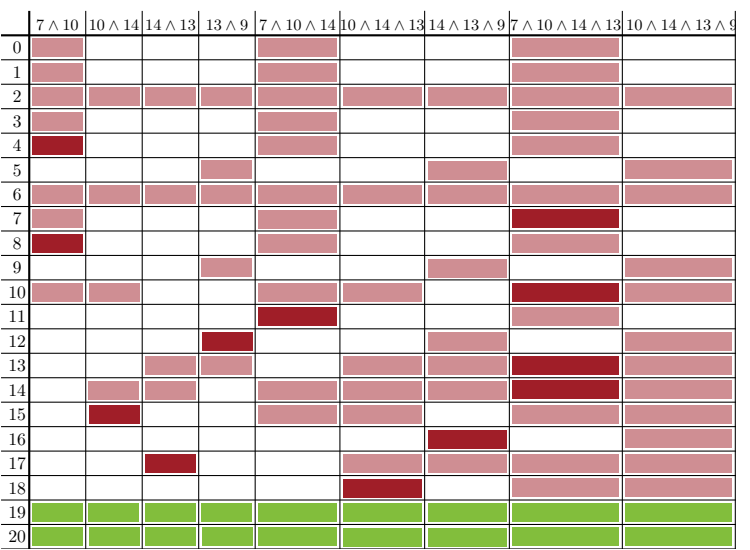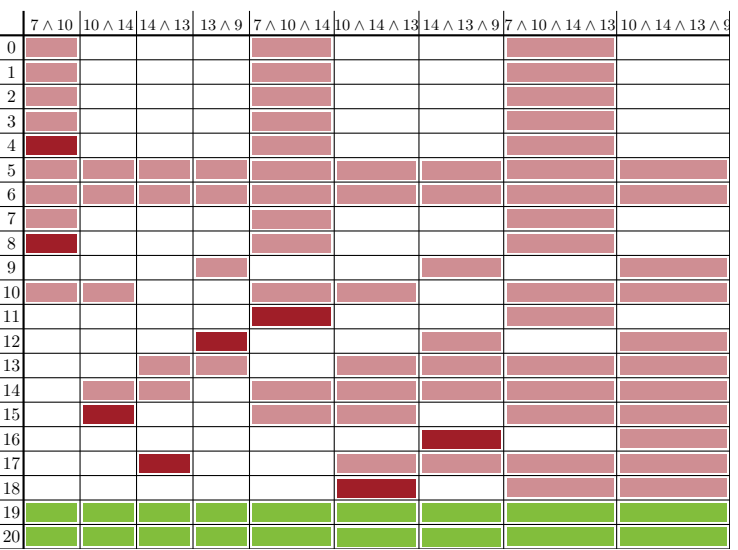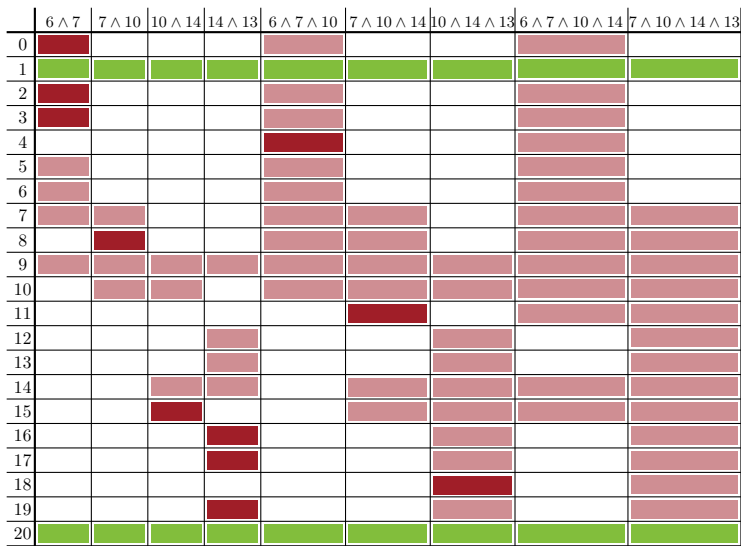

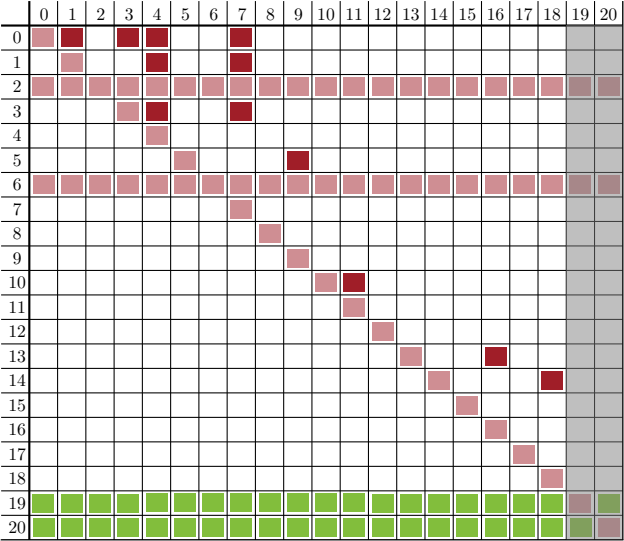

[illegible]

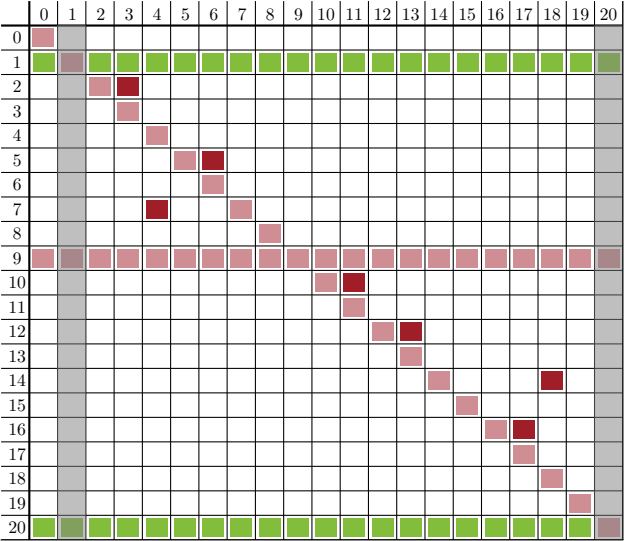



[illegible]

[illegible]

[illegible]

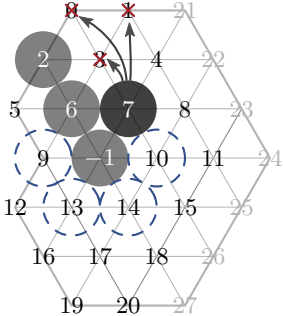

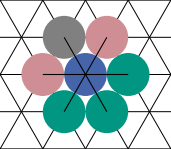

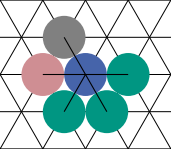

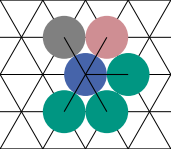

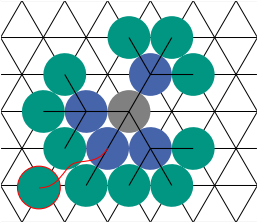



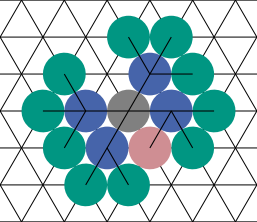

Supplement: Supplementary file 1 [file automated_appendix_details.pdf]
